# Supplementary material for: Metric Lines in Engel-type Groups
Source: arXiv:2405.08186 source file (2026-10-17)
Supplement: Supplementary file 1 [file Abnormal_Geodesics.tex]

\section{Abnormal Geodesics}\label{sub-AP:ab-geo}

\subsection{Proof of Lemma \ref{lemma:abn-geo-mag}}
\begin{proof}
We will compute the abnormal curves using the Pontryagin's maximum principle. Let us look the following optimal control problem:
\begin{equation}\label{eq:abn-proof-gama}
\dot{c}(t) = u_1 \tilde{X}_1 + \cdots + u_n \tilde{X}_n + u_{n+1} \tilde{Y}, 
\end{equation}
with the boundary conditions $\gamma(0)$ and $\gamma(T)$, we notice that equation \eqref{eq:abn-proof-gama} implies $\dot{x}_i = u_i$. It follows from Cauchy-Schwarz inequality that minimizing the \sR length is equivalent to minimizing the action
\begin{equation}\label{eq:abn-proof-gama-2}
\int_0^T \frac{u_1^2+ \cdots +u_{n+1}^2}{2}dt \to min,
\end{equation} 
with the condition $u_1^2 + \cdots + u_{n+1}^2 = 1$. Thus, the Hamiltonian associated to the optimal control problem \eqref{eq:abn-proof-gama} and \eqref{eq:abn-proof-gama-2} for the abnormal case is
\begin{equation}\label{eq:abn-proof-gama-3}
H(p,x,y,z,u) = u_1 p_{x_1} + \cdots +  u_n p_{x_n} + u_{n+1}(p_y + p_z F(x)). 
\end{equation}
From the Pontrygin's maximum principle, we obtain a Hamiltonian system for the variables $p_{x_1}, \cdots, p_{x_n}$, $p_y$ and $p_z$:
\begin{equation}\label{eq:abn-proof-gama-4}
\dot{p}_{x_i} = u_{n+1} \frac{\partial F}{\partial x_i}\;\;\text{for} \;\;i = 1,\dots,n,\;\;\dot{p}_y = 0 \;\;\text{and}\;\;\dot{p}_z = 0,
\end{equation}
the maximum condition
\begin{equation}\label{eq:pont-prin}
\max_{u \in \R^{n+1}} H(p(t),x(t),u) = H(p(t),\hat{x}(t),\hat{y}(t),\hat{z}(t),\hat{u}(t)), 
\end{equation}
where  $\hat{c}(t) = (\hat{x}(t),\hat{y}(t),\hat{z}(t))$ is the optimal process, and the condition of non-triviality $p(t) \neq 0$. Therefore, the maximum condition imply
\begin{equation}\label{eq:abn-proof-gama-5}
0 = p_{x_i}, \;\; \text{for} \;\;i = 1,\dots,n,\;\;\text{and}\;\; 0 = p_y + p_zF(x). 
\end{equation}
We notice that the non-trivial condition imply $(p_y,p_z) \neq (0,0)$, if $p_z = 0$, then $p_y = 0$, so $p_z \neq 0$. By derivating equation \eqref{eq:abn-proof-gama-5} with respect time and using equation \eqref{eq:abn-proof-gama-4}, we obtain;  
\begin{equation}\label{eq:abn-proof-gama-6}
0 = u_{n+1} \frac{\partial F}{\partial x_i}\;\;\text{for} \;\;i = 1,\dots,n,\;\;\text{and}\;\;  0 = \frac{\partial F}{\partial x_1} u_1 + \cdots + \frac{\partial F}{\partial x_n} u_n .  
\end{equation}
The left equation from \eqref{eq:abn-proof-gama-6} tells $u_{n+1} = 0$ or $\frac{\partial F}{\partial x_i} = 0$ for $i = 1,\dots,n$, this dichotomy yields the two different families of abnormal geodesics. 

\textbf{(Vertical lines)} Let us assume $\frac{\partial F}{\partial x_i} = 0$ for $i = 1,\dots,n$, then $u_1 = \cdots = u_n = 0$ since $F(x)$ is a quadratic function  and its unique critical point critical $x^*$ is isolated ($dF|_{x=x^*} = 0$. We conclude that $u_{n+1} = \pm 1$, so $c(t)$ is a vertical line.

\textbf{(Horizontal isocontour)}  Let us assume $u_{n+1} = 0$, then $c(t)$ is tangent to $\Ho$ and the second equation from \eqref{eq:abn-proof-gama-6} implies the curve $x(t)$ belongs to a level set of $F(x)$, a curve in the Euclidean sub-space $\Ho$ is a metric line if and only if is a line. 
\end{proof}

\subsection{Proof of Lemma \ref{lemma:abn-geo-Eng} }

\begin{proof}
Let us set up the notation $Y_i = [X_i,Y]$ and $Y_{n+1} = [X_i, y_i]$ for all $i=1,\dots,n$, where $\{X_1,\dots,X_n,Y\}$ is the frame for $\D$ presented in Section \ref{sec:Eng-type}. Following the strategy from the proof of Lemma \ref{lemma:abn-geo-mag}, we have 

\begin{equation}\label{eq:abn-proof-gama-3-En}
H(p,g,u) = u_1 P_{X_1} + \cdots +  u_n P_{X_n} + u_{n+1}P_{Y_0}, 
\end{equation}
where $P_{X_1}, \cdots ,P_{X_n}, P_{Y_0}$ are the left-invariant momentum function associated to the left-invariant vector fields tangent to $\Di$. From the Pontrygin's maximum principle, we obtain a Hamiltonian system for the left-invariant momentum functions:
\begin{equation}\label{eq:abn-proof-gama-4-En}
\begin{split}
\dot{P}_{X_i} & = -u_{n+1} P_{Y_i}\;\;\text{for} \;\;i = 1,\dots,n,\;\;\dot{P}_{Y_0} = u_1 P_{Y_1} + \cdots +  u_n P_{Y_n},\\
\dot{P}_{Y_i} & = u_{i} P_{Y_{n+1}}\;\;\text{for} \;\;i = 1,\dots,n,\;\text{and}\;\dot{P}_{Y_{n+1}} = 0. 
\end{split}
\end{equation}
 Then, the maximum condition imply
\begin{equation}\label{eq:abn-proof-gama-5-En}
0 = -u_{n+1} P_{Y_i} , \;\; \text{for} \;\;i = 1,\dots,n,\;\;\text{and}\;\; 0 = u_1 P_{Y_1} + \cdots +  u_n P_{Y_n}. 
\end{equation}

\textbf{(Vertical lines)} Let us consider the case $P_{Y_1} = \cdots = P_{Y_n} = 0$, the no trivial condition implies $P_{Y_{n+1}} \neq 0$. Since $P_{Y_1}, \cdots, P_{Y_n}$ are constant, then equation \eqref{eq:abn-proof-gama-4-En} says  $0 = u_{i} P_{Y_{n+1}}$ for $i = 1,\dots,n$, so $0 = u_{i}$ for $i = 1,\dots,n$. We conclude that $u_{n+1} = \pm 1$, so $\gamma(t)$ is a vertical line. 

\textbf{(Horizontal curves)} Let us consider the case $P_{Y_{n+1}} = 0$, then \eqref{eq:abn-proof-gama-4-En} and the non-trivial condition show $(P_{Y_1}, \cdots, P_{Y_n})$ is a constant vector different of zero. Therefore, the \eqref{eq:abn-proof-gama-5-En} implies $u_{n+1} = 0$ and  $(P_{Y_1}, \cdots, P_{Y_n})\cdot (u_1, \cdots,u_n) = 0$, so $\gamma(t)$ is a Horizontal curve tangent to $\Ho$ and perpendicular to the vector $(P_{Y_1}, \cdots, P_{Y_n})$.

Let us consider the case $P_{Y_{n+1}} \neq 0$, then equation \eqref{eq:abn-proof-gama-4-En} yields $u_i = \frac{\dot{P}_{Y_i}}{P_{Y_{n+1}}}$, plugin the last expression \eqref{eq:abn-proof-gama-5-En} implies
$$ 0 = \dot{P}_{Y_1} P_{Y_1} + \cdots +  \dot{P}_{Y_n} P_{Y_n}\;\;\text{then}\;\; R^2 = P^2_{Y_1} + \cdots +  P^2_{Y_n}. $$
We conclude that $(P_{Y_1}, \cdots, P_{Y_n})$ is never the zero vector if $R \neq 0$, so $u_{n+1} = 0$, and $\gamma(t)$ is tangent to a sphere in $\Ho$. If $R = 0$, then $\gamma(t)$ is vertical line.

\end{proof}
