# Supplementary material for: Metric Lines in Engel-type Groups
Source: arXiv:2405.08186 source file (2026-10-17)
Supplement: Supplementary file 2 [file sequence-method-apendix.tex]

\section{Sequence Method}

\subsection{Sequence Method for direct-type Geodesics}

Let us present the theorem for direct-type geodesics. 
\begin{Theorem}[Sequence method for direct-type gedesic]\label{the:metrtic-lines-method-d-t}
Let $\G$ be a \ma Carnot group with a semidirect product structure such that $\dim \; \Vs = 1$. Let $\gamma_d(t)$ be a directy-type geodesic in $\G$ corresponding to a polynomial $F(x)$, and let $c_d(t):= \pi_F(\gamma_s(t))$ be the \sR geodesic in $\R^{n+2}_F$. Without loss of generality, let us assume that $[c_d]$ is in $Hetc^+(x_0,x_1)$. If the following conditions hold: 
\begin{enumerate}
\item The value $\Theta_1([c_d])$ is finite. 
\item  There exist a ball $B_{\Ho}$ with the property that the region $B_{\Ho}(r,x_0) \times \R^{2}$ is geodesically compact.

\item The map $\Theta_2: Hetc^+(x_0,x_1) \to \R$ is one to one.

\item  The sequence of minimizing geodesics $c_n(t)$ joining the points $c(-n)$ and $c(n)$ is strictly normal. 

\end{enumerate}
Then $c_d(t)$ is a metric line in $\R^{n+2}_F$, consequently the direct-type geodesic $\gamma_d(t)$ is a metric line. 
\end{Theorem}

We will omit the proof of Theorem \ref{the:metrtic-lines-method-d-t} since it follows the same strategy. See \cite{bravo2022metric} for the jet space case.

\subsection{Complementary Results for the Sequence Method for Homoclinic Geodesics}

An essential definition for this section is the following.

\begin{defi}
Let us consider the vector space of polynomial on $\R$  of degree bounded by $k$, and let  $||F||_{\infty} :=  \sup_{x \in [0,1]} |F(x)|$ be the uniform norm. We denote by $\mathcal{P}(k)$ the closed ball of radius 1.
\end{defi}

We remark that it is well-known that $\mathcal{P}(k)$ is a compact set. This result will be fundamental for the following proof.

\subsubsection{Proof of Lemma \ref{lem:uniform-bound-c-n} }\label{app:lem-unif-bounf-c-n}

We will devote this section to prove Lemma \ref{lem:uniform-bound-c-n}. The strategy is the following: We will consider a magnetic space $\R^{n+1}_F$ with a geodesically compact region $B_{\Ho}(r,x_0)\times \R^2$. We will take the map $Cost_y(c,\mathcal{T})$ restricted to the space $Com(r,x_0,C)$. For every pair $(c,\mathcal{T})$, we will associate a pair $(G,x(\mathcal{T}))$ and we will take on $Cost_y(c,\mathcal{T})$ as a function on the space on the space of pairs $(G,x(\mathcal{T}))$. Then, we will show that the map $Cost_y(c,\mathcal{T})$ is a continuous function restricted to the space  $Com(r,x_0,C)$, i.e., we will consider a sequence of pairs $(G_n,x_n(\mathcal{T_n}))$ converging to $(G,x(\mathcal{T}))$ and show that $Cost_y(c_n,\mathcal{T}_n)$ converge to $Cost_y(c,\mathcal{T})$. We will show that the sequence of pairs defined by Lemma \ref{lem:uniform-bound-c-n} is sequentially compact. Therefore, $Cost_y(c,\mathcal{T})$ is a continuous function on a sequentially compact set, so $Cost_y(c,\mathcal{T})$ is bounded.

An essential result of this proof is the General Lebesgue Dominated Convergence Theorem.

\begin{Theorem}[General Lebesgue Dominated Convergence Theorem]
Let $\{f_n\}$ be a sequence of measurable functions on $E$ that converge pointwise a.e. on $E$ to $f$. Suppose there is a sequence $\{g_n\}$ of nonnegative functions on $E$ that converges a.e. on $E$ to $g$ and dominates $\{f_n\}$ on $E$ in the sense that
$$|f_n| \leq g_n \;\;\text{on}\;\;E\;\; \text{for all}\;\;n.$$
$$\text{If}\;\;\lim_{n\to \infty} \int_{E} g_n = \int_{E} g< \infty,\;\;\text{then}\;\; \lim_{n\to \infty} \int_{E} f_n = \int_{E} f.$$
\end{Theorem}

\begin{Prop}\label{prp:cost-cont}
    Let $\R^{n+1}_F$ be magnetic space, and let $B_{\Ho}(r,x_0)\times \R^2$ be a geodesically compact region. Then, the function $Cost_y(c,\mathcal{T})$ is continuous in the space $Com(r,x_0,C)$. 
\end{Prop}
We remark that if $c(t)$ is a \sR geodesic corresponding to a polynomial $G(x)\in Pen_F$, then we think on $Cost_y(c,\mathcal{T})$ as a function on the polynomial $G(x)$ and the curve $x(\mathcal{T})$. Let us prove Proposition \ref{prp:cost-cont}.  
\begin{proof}
    We will consider a sequence $(c_n,\mathcal{T}_n) \in Com(r,x_0,C)$ converging to a pair $(c,\mathcal{T})$, and we will show that 
    $$\lim_{n\to \infty}Cost_y(c_n,\mathcal{T}_n) = Cost_y(c,\mathcal{T}). $$
    The goal is to apply G.L.D.C.T. (General Lebesgue Dominated Convergence Theorem). Let us consider the following cases.
    
    (Case 1) The interval $\mathcal{T}$ is bounded. We will use $E = \R$, and we define the sequence of functions $\{f_n\}$ and $\{g_n\}$ as follows
    \begin{equation*}
        \begin{split}
     f_n(t)& = \begin{cases}
              G_n(x_n(t))(1-F(x_n(t)) \quad \text{if}\;\;t \in \mathcal{T}_n,\\
              0 \qquad\qquad\qquad\qquad\;\;\;\qquad \text{if}\;\;t \notin \mathcal{T}_n,
             \end{cases}\\    
      g_n(t)& = \begin{cases}
              C_F \quad \text{if}\;\;t \in \mathcal{T}_n,\\
              0 \quad\;\;\; \text{if}\;\;t \notin \mathcal{T}_n,
             \end{cases} \quad\text{where}\quad C_F:= \max_{x\in K_{\Ho}} (1-F(x)).\\        
        \end{split}
    \end{equation*}
By construction, we have $|f_n| \leq g_n$. We define the functions $f$ and $g$ by
\begin{equation*}
        \begin{split}
     f(t)& = \begin{cases}
              G(x(t))(1-F(x(t)) \quad \text{if}\;\;t \in \mathcal{T},\\
              0 \qquad\qquad\qquad\;\;\;\;\qquad \text{if}\;\;t \notin \mathcal{T},
             \end{cases}\;\;\text{and}\;\;    
      g(t) = \begin{cases}
              C_F \quad \text{if}\;\;t \in \mathcal{T},\\
              0 \quad\;\;\; \text{if}\;\;t \notin \mathcal{T}.
             \end{cases}\\        
        \end{split}
    \end{equation*}
    Since the Lebesgue measure of the interval $\mathcal{T}_n$ is finite for all $n$ and the one for interval $\mathcal{T}$, we can apply G.L.D.C.T. to obtain our desired result.

    (Case 2) The interval $\mathcal{T}$ is unbounded. Without loss of generality, let us assume that $\mathcal{T} = [-\infty,\infty]$ (otherwise, we repeat the proof with only one side unbounded).  We define the following sets
    $$\mathcal{T}^+_n := \{ t \in \mathcal{T}_n: \; 0 < G(x(t))  \}\;\;\text{and}\;\; \mathcal{T}^-_n := \{ t \in \mathcal{T}_n: \; 0 > G(x(t))  \} .$$
    Let us notice that $Cost(c_n,\mathcal{T})$ is uniformly bounded implies that the Lebesgue measure of $\mathcal{T}^-_n$ is uniformly bounded for all $n\in \mathbb{N}$. Indeed,
    \begin{equation*}
        \int_{\mathcal{T}^-_n} dt \leq \int_{\mathcal{T}^-_n} (1-G_n(x_n(t))) dt < C.  
    \end{equation*}

    Since $c_n(t)$ is a sequence of minimizing geodesic, Proposition \ref{prop:conj-point} implies that $c(t)$ can touch only once the boundary $\Omega^+_{G_n}$ in the interior of the interval $\mathcal{T}_n$, or twice in the bounder of the interval $\mathcal{T}_n$. Having this in mind and assuming that $\mathcal{T}_n = [(t_0)_n,(t_1)_n]$, we define the following set
    $$ \mathcal{T}_n^1 := \{ [(t_0)_n,(t_0)_n+1]\cup [t^*-\epsilon,t^*+\epsilon] \cup [(t_1)_n-1,(t_1)_n+1]\subset\mathcal{T} : \;\; G_n(t^*) =1 \},   $$
    where $\epsilon$ is any positive number that make us sure that $\T_n^1 \subset \T_n$ for $n\in \mathbb{N}$, where we are assuming that $t^*_n$ converge to a real number when $n\to \infty$, we will consider the opposite later. We remark that Lemma \ref{lem:com-converge} implies that 
    $$ \lim_{n\to \infty}G(x((t_0)_n) = \lim_{n\to \infty}G(x((t_1)_n) = 1.$$
    Since $x((t_0)_n \to -\infty$ and $x((t_1)_n \to \infty$ when $n \to \infty$. Consequently, 
    \begin{equation*}
        \lim_{n\to \infty}G(x((t_0)_n+1) = \lim_{n\to \infty}G(x((t_1)_n-1) = 1.
    \end{equation*}
    We define the interval $\mathcal{T}^1$ as the limit of $\T^1_n$ when $n \to \infty$ given by
    $$ \T^1:= \{  [t^*-\epsilon,t^*+\epsilon] \subset\mathcal{T} : \;\; G_n(t^*) =1 \} $$
    
    We use the set $\T_n^1$ to rewrite the following integral
    \begin{equation*}
        \begin{split}
        \int_{\mathcal{T}^+_n} G_n(x_n(t))(1-F(x_n(t))) dt = & \int_{\mathcal{T}^1_n} G_n(x_n(t))(1-F(x_n(t))) dt\\
         & +  \int_{s(\T_n\setminus\mathcal{T}^1_n)} \frac{G_n(x_n(s))(1-F(x_n(s)))}{\sqrt{1-G^2_n(x_n(s))}}ds.
        \end{split}
    \end{equation*}

    For all $n \in \mathbb{N}$, we define the interval $\overline{\T}_n = \T^- \cup \T^1_n$ and the sequences functions  $\{f_n^1\}$ and $\{g_n^1\}$ on the interval $\R$ as follows
    \begin{equation*}
        \begin{split}
     f_n^{1}(t)& = \begin{cases}
              G_n(x_n(t))(1-F(x_n(t)) \quad \text{if}\;\;t \in \overline{\T}_n,\\
              0 \qquad\qquad\qquad\qquad\;\;\;\qquad \text{if}\;\;t \notin \overline{\T}_n,
             \end{cases}\;\text{and}\;\;    
      g_n^{1}(t) = \begin{cases}
              C_F \; \text{if}\;t \in \overline{\T}_n,\\
              0 \quad \text{if}\;t \notin \overline{\T}_n.
             \end{cases}\\        
        \end{split}
    \end{equation*}
    By construction, we have $|f_n^1| \leq g_n^1$ for all $n \in \mathbb{N}$. We define $\overline{\T} = \T^- \cup \T^1$ and the functions $f^1$ and $g^1$ on $\R$ by
\begin{equation*}
        \begin{split}
     f^1(t)& = \begin{cases}
              G(x(t))(1-F(x(t)) \quad \text{if}\;\;t \in \overline{\T},\\
              0 \qquad\qquad\qquad\;\;\;\;\qquad \text{if}\;\;t \notin \overline{\T},
             \end{cases}\;\;\text{and}\;\;    
      g^1(t) = \begin{cases}
              C_F \quad \text{if}\;\;t \in \overline{\T},\\
              0 \quad\;\;\; \text{if}\;\;t \notin \overline{\T}.
             \end{cases}\\        
        \end{split}
    \end{equation*}
    The function $ g^1$ is integrable since the Lebesgue measure of $\overline{\T}_n$ is uniformly bounded. Therefore, the sequences of functions $ \{f^1_n\}_{n\in \mathbf{N}}$ and $\{g^1_n\}_{n\in \mathbf{N}}$ satisfy the hypothesis of G.L.D.C.T.

    For every $s \in S(\T_n\setminus\mathcal{T}^1_n)$, we have that
    $$ \frac{G_n(x_n(s))(1-F(x_n(s)))}{\sqrt{1-G^2_n(x_n(s))}} $$
    is a smooth function. Moreover, $S(\T_n\setminus\mathcal{T}^1_n)$ is a compact set, then there exists a constant $C_n^*$ defined by
    $$ C_n^*:= \max_{s\in S(\T_n\setminus\mathcal{T}^1_n)}\frac{|1-F(x_n(s))|}{\sqrt{1-G^2_n(x_n(s))}} .  $$
    Lemma \ref{lem:com-converge} implies that
    $$ \lim_{n\to \infty}\Big|\frac{G_n(x_n(s))(1-F(x_n(s)))}{\sqrt{1-G^2_n(x_n(s))}}\Big| = 0\;\;\text{for all}\;\;s\in S(\mathcal{T}^1_n\setminus[t^*_n-\epsilon,t^*_n+\epsilon]).  $$
    We concluded that
    $$C^*:=\lim_{n \to \infty} C^*_n = \max_{s\in S(\T\setminus\mathcal{T}^1)}\frac{|1-F(x(s))|}{\sqrt{1-G^2(x(s))}}.$$
    When $t^*_n$ diverges we define $C^* := 0$. 

   The arc-length of $x_n(t)$ is uniformly bounded by $S_0$ by Definition \ref{def:geo-comp-def}. We define the interval $\overline{S}_n := s(\T_n\setminus\mathcal{T}^1_n) \cap [0,S_0]$, and the sequences functions  $\{f_n^2\}$ and $\{g_n^2\}$ on the interval $[0,S_0]$ as follows
    \begin{equation*}
        \begin{split}
     f_n^{2}(s)& = \begin{cases}
              \frac{G_n(x_n(s))(1-F(x_n(s)))}{\sqrt{1-G^2_n(x_n(s))}} \; \text{if}\;\;s \in \overline{S}_n,\\
              0 \qquad\qquad\qquad \;\;\;\;\;\;\;\;\text{if}\;\;s \notin \overline{S}_n,
             \end{cases}\;\text{and}\;  
      g_n^{2}(s) = \begin{cases}
              C_n^* \; \text{if}\;s \in \overline{S}_n,\\
              0 \quad \text{if}\;s \notin \overline{S}_n.
             \end{cases}\\        
        \end{split}
    \end{equation*}
    By construction, we have $|f_n^1| \leq g_n^1$ for all $n \in \mathbb{N}$.  If $t_n^*$ converges, we define $\overline{S} = s([t^*-\epsilon,t^*+\epsilon])\cap [0,S_0]$, if $t^*_n$ does not converges we define $\overline{S}$ as the empty set. We define the functions $f^2$ and $g^2$ on the interval $[0,S_0]$ by
    \begin{equation*}
        \begin{split}
     f^{2}(s)& = \begin{cases}
              \frac{G_n(x(s))(1-F(x(s)))}{\sqrt{1-G^2(x_n(s))}} \; \text{if}\;\;s \in \overline{S},\\
              0 \qquad\qquad\qquad \;\;\;\text{if}\;\;s \notin \overline{S},
             \end{cases}\;\;\text{and}\;  
      g^{2}(s) = \begin{cases}
              C^* \; \text{if}\;s \in \overline{S},\\
              0 \quad \text{if}\;s \notin \overline{S}.
             \end{cases}\\        
        \end{split}
    \end{equation*}
    The function $ g^2$ is integrable since the Lebesgue measure of $\overline{S}$ is bounded. Therefore, the sequences of functions $ \{f^2_n\}_{n\in \mathbf{N}}$ and $\{g^2_n\}_{n\in \mathbf{N}}$ satisfy the hypothesis of G.L.D.C.T. By construction, we have
    $$ Cost_y(c_n,\T_n) = \int_{\R} f^1_n(t) dt + \int_{[0,S_0]} f^2_n(s)ds.$$
    Therefore, G.L.D.C.T. implies that $Cost_y(c_n,\T_n) \to Cost_y(c,\T)$ when $n\to \infty$. 
\end{proof}

We are ready to prove Lemma \ref{lem:uniform-bound-c-n}.

\begin{proof}
Let us consider the pairs $(c_n,[0,t_n^*])$. Since $c_n(t)$ is a normal sequence, we can associate each pair $(c_n,[0,t_n^*])$ with a pair $(G_n,x_n([0,t_n^*]))$. The goal is to show that the sequence $(G_n,x_n([0,t_n^*]))$ is sequatially compact. 

Since $c_n(t)$ is a normal sequence, the Hill region $\Omega_{G_n}$ is not a singleton so we can find a ball $B_{\Ho}(\epsilon_n,x_n)\subset \Omega_{G_n}$, where we impose $\epsilon_n\leq 1$. We consider the affine map $h_n(\tilde{x}) = x_n + \epsilon_n \tilde{x}$, which maps $B_{\Ho}(1,0)$ to $B_{\Ho}(\epsilon_n,x_n)$. Then, we consider the sequence of polynomials $\widehat{G}_n(\tilde{x}):= G_n(h_n(\tilde{x})$. Therefore, $\widehat{G}_n(\tilde{x}) \in \mathcal{P}(s-1)$, where $s$ is the step of the Carnot group $\G$ and we concluded that there exist a convergent subsequence $\widehat{G}_{n_j}(\tilde{x})$ . Moreover, we find a convergent subsequence of maps $h_{n_j}$ since $x_n \in K_{\Ho}$ and $\epsilon_n \in [0,1]$. Then, we find a convergent subsequence of polynomials  $G_{n_j}(x)$.

The sequence of polynomials $G_n(x)$ defines a sequence of Hamiltonian systems with an initial condition $x_n(0) \in K_{\Ho}$. Therefore, the subsequence of polynomials  $G_{n_j}(x)$ defines a convergent subsequence of Hamiltonian systems with a convergent subsequence of initial conditions. Then, we extract a convergent subsequence of curves $x_{n_j}([0,t^*_{n_j}])$. The map   $Cost_y(c_n,[0,t^*_n])$ is a continuous function restricted to a sequentially compact set, then $Cost_y(c_n,[0,t^*_n])$ is uniformly bounded. 
\end{proof}

\subsubsection{Proof of Lemma \ref{lem:geod-com-Ent} } \label{ap:proof-geod-com-Ent}

Let us prove Lemma \ref{lem:geod-com-Ent}.

\begin{proof}
%Let $c_n(t) = (x_n(t),y_n(t),z_n(t))$ be a sequence of geodesic in $\R^{n+2}_F$ with $F(r) = 1 - br^2$ traveling during a time interval $\mathcal{T}_n$ such that $x_n(\partial\mathcal{T}_n)$ is in $B_{\Ho}(r)$ for all $n$. We will prove that if $\mathcal{C}_n$ is unbounded, then $Cost(c_n,\mathcal{T}_n)$ is unbounded.

Let us consider the ball $B_{\Ho}(r^*,0)\subset\Ho$ for arbitrary radius $r_0$. Let $(c_n,\mathcal{T}_n)$ be a sequence of geodesic in $Com(r^*,0,C)$ where $c_n(t) = (x_n(t),y_n(t),z_n(t))$ is a geodesic in $\R^{n+2}_F$ with $F(r) = 1 - 2r^2$ and $\mathcal{T}_n$ is time interval sequence such that $\mathcal{T}_n \to [-\infty,\infty]$, where $n \to \infty$. We will prove first that the radial interval $r(\mathcal{T}_n) = [(r_{min})_n,(r_{max})_{n}]$ is uniformly bounded and then we will see that length of $s(\mathcal{T}_n)$ is uniformly bounded.

%First let us rewrite the $Cost_t(c_n,\mathcal{T}_n)$ as follows
% \begin{equation*}
%     Cost(c_n,\mathcal{T}_n) = \int_{r(\mathcal{T}_n)} \frac{r(1-G_n(r)) dr}{\sqrt{r^2(1-G_n^2(r)) - \ell_n^2}}.
% \end{equation*}
For the first part, we will show that if $x_n(\mathcal{T}_n)$ is unbounded, then $Cost(c_n,\mathcal{T}_n)$ is unbounded. 
The sequence of geodesics $c_n(t)$ induces a sequence of pairs $(G_n,\ell_n)$. The first goal is to extract a convergent subsequence  $(G_{_j},\ell_{n_j})$.  If $r(\mathcal{T}_n) = [(r_{min})_n,(r_{max})_{n}]$, we consider the affine map $h_n(\tilde{r}) = (r_{min})_n + u_n \tilde{r}$ with $u_n := (r_{max})_n - (r_{min})_n$, which maps $[0,1]$ to $r(\mathcal{T}_n)$. Since the effective potential satisfies $ V_n(r) = \frac{\ell_n^2}{r^2} + G^2_n(r) \leq 1$, it follows that the polynomial  $\tilde{G}_n(\tilde{r}) = G_n^2(h_n(\tilde{r}))$ is in $\mathcal{P}(6)$. Moreover, the condition $x_n(t)$ leaves the ball $B_{\Ho}(r^*,0)$ for some $t$ in $\mathcal{T}_n$ implies $|\ell_n| < r^*$, then $\ell_n$ is a sequence of bounded real numbers. Therefore, there exists a subsequence $(\tilde{G}_{n_j},\ell_{n_j})$ converging to $(\tilde{G},\ell)$. Let us proceed by the following cases: case $\tilde{G}(\tilde{r}) \neq 1$ and case $\tilde{G}(\tilde{r}) = 1$.

Case $\tilde{G}(\tilde{r}) \neq 1$: setting the change of variable, $r = h_{n_j}(\tilde{r})$, we have
$$ Cost_t(c_n,\mathcal{T}_n) = u_n \int_{[0,1]} \frac{1-\tilde{G}_{n_j}(\tilde{r})}{\sqrt{1-\frac{\ell^2_{n_j}}{\tilde{r}^2} - \tilde{G}^2_{n_j}(\tilde{r})}} d\tilde{r} , $$
Therefore, Fatou's lemma implies
$$ 0 <\int_{[0,1]} \frac{1-\tilde{G}(\tilde{r})}{\sqrt{1-\frac{\ell^2}{\tilde{r}^2} - \tilde{G}^2(\tilde{r})}} d\tilde{r} \leq \liminf_{n_j \to \infty}  \int_{[0,1]} \frac{1-\tilde{G}_n(\tilde{r})}{\sqrt{1-\frac{\ell^2_{n_j}}{\tilde{r}^2} - \tilde{G}^2_{n_j}(\tilde{r})}} d\tilde{r} .$$
Then, $u_{n_j} \to \infty$ implies $Cost_t(c_{n_j},\mathcal{T}_{n_j})$ when $n_j \to \infty$.

Case  $\tilde{G}(\tilde{r}) = 1$: there exist $n^*$ such that $\tilde{G}_{n_j}(\tilde{r}) > \frac{1}{2}$ for all $\tilde{r}$ in $[0,1]$ if $n_j > n^*$, so $\frac{3}{4} \leq 1-\frac{\ell_{n_j}^2}{r^2} - G_{n_j}^2(\tilde{r}) $. Using that $1-F(r) = 2r^2$, then we have
\begin{equation*}
\begin{split}
\frac{2 u_{n_j}}{\sqrt{3}}  & \int_{[0,1]} r^2dr <  Cost_y(G_{n_j},\mathcal{T}_{n_j}) . \\
\end{split}
\end{equation*} 
So $ Cost_y(G_{n_j},\mathcal{T}_{n_j})\to \infty$, when $n_j \to \infty$. Therefore, we conclude that the radial interval  $r(\mathcal{T}_n)$ is uniformly bounded, i.e., there exists a $C_r$ such that 
$$ \max_{n\in \mathbb{N}}\{r(\mathcal{T}_n)\} < C_r.$$

If $\ell_n = 0$, Proposition \ref{Maxwell-r} implies $s(\mathcal{T}_n)<2C_r$. If $\ell_n \neq 0$ and $r_n(t)$ is constant, i.e., it is a relative equilibrium point by Lemma \ref{lemma:equi-point-an-har}, then  Proposition \ref{Maxwell-r} implies $s(\mathcal{T}_n)<2\pi C_r$. 

We will focus on the case when $\ell_n \neq 0$ and $r_n(t)$ is not constant. We can think of the one-form, defining the change in the coordinate $\theta$ given by equation \ref{eq:theta-period}, as a smooth, closed, and not exact one-form defined on the closed and simple curve on the plane $(r,p_r)$ given by the equation
$$ \alpha_n  := \{(p_r,r) \in \R^2: \frac{1}{2} = H_{n}(p_r,r) := \frac{1}{2} \big(p_r^2 + \frac{\ell_n^2}{p_r^2} + G_n^2(r)\big),\;\text{and}\; r \in \mathcal{R}_n   \}.  $$
This one-form is given by
$$ \phi_n =\frac{2\ell_ndr}{r^2\sqrt{1-V_n(r)}},\;\text{and the change by}\;\Delta\theta(c_n,\mathcal{T}_n) = \int_{r(\mathcal{T}_n)} \frac{2\ell_ndr}{r^2\sqrt{1-V_n(r)}}. $$
Note that $\ell_0\neq 0$ implies $0 \notin \mathcal{R}_n$.

We will proceed as in \cite[Lemma A.4]{bravo2022metric}. Our goal is to show that $\Delta\theta(c_n,\mathcal{T}_n)$ is uniformly bounded by a constant $C_\theta$. If this is true, then the arc length of the curve $s(\mathcal{T}_n)$ is bounded by $C_rC_\theta$.

Indeed, by the preimage theorem, the curve $\alpha_n$ is smooth at a point $(p_r,r) \in \alpha_n$ if and only if $\nabla H_n(p_r,r) \neq 0$ if and only if $(p_r,r)$ is a relative equilibrium point, but this is not the case. Therefore, $\alpha_n$ is smooth. It is well known that the one-form is smooth around a neighborhood of the parameters $\ell_n, a_n$, and $b_n$ where the curve $\alpha_n$ is smooth, see \cite[Remark 2.21]{bravo2022metric}, \cite[Lemma 2.24]{bravo2022metric}, or \cite[Chpater 3.10]{lawden2013elliptic}. 

To find $C_{\theta}$, we proceed in two steps: first, the smoothness of the one-form $\phi_n$ implies that $h^*_n\phi_n$ is smooth, where $h_n^*$ is the pull back of $h_n(\tilde{x})$. We fix the lower bound of the integral $h_n^{-1}(r(0))$ and vary the upper bound $h_n^{-1}(r(t))$, where $r \in \mathcal{T}_n$. The integral of $h^*_n\phi_n$ is a smooth function with respect to the upper bound $h_n^{-1}(r(t))$, and we can find its maximum
$$ \max_{h_n^{-1}(r(t)) \in [0,1]} \big|\int_{h_n^{-1}([0,t])} h^*_n\phi_n\big|.$$
Second,  the above value is smooth with respect to the parameters $\ell_n, a_n$, and $b_n$, and they belong to a sequentially compact set, then the above value is uniformly bounded for all $n \in \mathbb{N}$.

\end{proof}
